# Supplementary material for: Dichotomy of Early and Late Phase Implicit Biases Can Provably Induce Grokking
Source: arXiv:2311.18817 source file (2024-04-02)
Supplement: Supplementary file 1 [file appendix_margin.tex]

\begin{comment}
\subsection{Dynamical Analysis of the Linearized Model}

We focus on the dynamics of the linearized model $\vthetalin(t; \vtheta_0)$ with $\vtheta_0 = \vthetauinit$. For this initialization, we have

%which can be simplified to $\flin_i(\vtheta; \vtheta_0) = \inner{\vtheta}{\nabla f_i(\alpha \vthetauinit)}$ when the initial point $\vtheta_0$ is set to $\alpha \vthetauinit$ (see \Cref{sec:prelim}).

This is because the property $\forall \alpha, i: f_i(\alpha\vthetauinit) = 0$ can be applied to simplify the linearized model as $\flin_i(\vtheta; \vtheta_0) = f_i(\vtheta_0) + \inner{\vtheta - \vtheta_0}{\nabla f_i(\vtheta_0)} = \inner{\vtheta}{\nabla f_i(\vtheta_0)}$ when $\vtheta_0 = \alpha \vthetauinit$, thanking to the homogeneity $\inner{\vtheta_0}{\nabla f_i(\vtheta_0)} = 2 f_i(\vtheta_0) = 0$. 
\begin{align*}
    \cLlin(\vtheta; \alpha \vthetauinit) = \frac{1}{n} \sum_{i=1}^{n} \ell(y_i \inne{\vtheta}{\nabla f_i(\alpha \vthetauinit)}).
\end{align*}

Then it is clear that training the linearized model $\flin_i$ leads to the same trajectory as training linear 

\end{comment}

\subsection{Proof for Theorem~\ref{thm:diag-net-chizat-ntk}}

\subsection{Proof for Theorem~\ref{thm:1-sparse-grokking}}

\begin{proof}
    Let $\beta := (1 + c)M \log M$.
    
    KKT:
    \begin{align*}
        &\hat{w}_k = \frac{2}{\beta} \sinh\left(\sum_{i=1}^{n} \lambda_i y^*_i x_{i,k} \right) \\
        & \inner{y^*_i \vx_{i}}{\hat{\vw}} = 1 \quad \text{or} \quad \lambda_i = 0. \\
        & \inner{y^*_i \vx_{i}}{\hat{\vw}} \ge 1 \\
        & \lambda_i \ge  0.
    \end{align*}

    Let $S := \sum_{i=1}^{n} \lambda_i$. 

    For $k=1$, $\hat{w}_1 = \frac{2}{\beta} \sinh(S)$.

    $\bar{Q}(\sinh(S)) = \bar{Q}(\frac{\beta}{2} \hat{w}_1) \le Q_{2/\beta}(\hat{\vw}) \le Q_{2 / \beta}\left((1, 0, \dots, 0)\right) = \bar{Q}(\frac{\beta}{2})$.

    So $S \le \arcsinh \frac{\beta}{2} = \cO(\log d)$.
    
    For $2 \le k \le d$, $\abs{\sum_{i=1}^{n} \lambda_i y^*_i x_{i,k}} \le \sum_{i=1}^{n} \lambda_i \epsilon_0 = S \epsilon_0 = \cO(\epsilon_0 \log d)$. Since $\epsilon_0 \log d = o(1)$, by Taylor expansion of $\sinh$ we have
    \begin{align*}
        \frac{\beta}{2}\hat{w}_k = \sum_{i=1}^{n} \lambda_i y^*_i x_{i,k} + \cO(\epsilon_0^2 \log^2 d).
    \end{align*}

    For all $i \in [n]$,
    \begin{align*}
        \frac{\beta}{2} \le \frac{\beta}{2} \inner{\hat{\vw}}{y_i\vx_i} &= \sinh(S) +  \sum_{j=1}^{n} \lambda_j  \sum_{k=2}^{d}y^*_j x_{j,k} \cdot y^*_i x_{i,k} + \cO(\epsilon_0^3 d \log^2 d) \\
        &=\sinh(S) + \lambda_i \epsilon_0^2 (d-1) +  \sum_{j \ne i} \lambda_j  \cdot \cO\left(\epsilon_0^2\sqrt{d \log(n/\delta)}\right) + \cO(\epsilon_0^3 d \log^2 d) \\
        &=\sinh(S) + \lambda_i \epsilon_0^2 (d-1) + \cO\left(\epsilon_0^2 \log d\sqrt{d \log(n/\delta)} + \epsilon_0^3 d \log^2 d\right)
    \end{align*}
    Averaging over support vectors gives
    \begin{align*}
        \frac{\beta}{2} + \cO\left(\epsilon_0^2 \log d\sqrt{d \log(n/\delta)} + \epsilon_0^3 d \log^2 d\right) &= \sinh(S) + \frac{\epsilon_0^2 (d-1)}{m} \cdot S. \\
    \end{align*}
    So
    \begin{align*}
        S &\le \frac{m}{\epsilon_0^2 (d-1)} \cdot \frac{\beta}{2} + \cO\left( \frac{n\epsilon_0^2}{\sqrt{d}} \log d \sqrt{\log(n/\delta)}+ n\epsilon_0 \log^2 d\right) \\
        &= (1+c) \cdot \frac{m}{n} \cdot \frac{1}{2} \log M + \cO(1) \\
        &\le \frac{1+c}{2} \log M + \cO(1).
    \end{align*}
    So
    \begin{align*}
        \sinh(S) \le \cO\left(\exp\left(\frac{1+c}{2}\log M + o(1)\right)\right) = \cO(M^{(1+c)/2}).
    \end{align*}
    Solve for $\lambda_i$.
    \begin{align*}
        \lambda_i &= \frac{1}{\epsilon_0^2 (d-1)} \left( \frac{\beta}{2} - \sinh(S)  \right) + \cO\left( \frac{1}{\sqrt{d}} \log d \sqrt{\log(n/\delta)} +\epsilon_0 \log^2 d\right) \\
        &= \frac{1}{\epsilon_0^2 (d-1)} \cdot \frac{\beta}{2} + \frac{1}{n} \left(  \cO( M^{-(1-c)/2}) + \cO(1)\right) \\
        &= \frac{1}{n}\left(
        \frac{1 + c}{2} \log M + \cO(1)
        \right) > 0.
    \end{align*}
    So $m = n$. Then
    \begin{align*}
        S &= \frac{n}{\epsilon_0^2 (d-1)} \cdot \frac{\beta}{2} + \cO( M^{-(1-c)/2}) + \cO\left( \frac{n\epsilon_0^2}{\sqrt{d}} \log d \sqrt{\log(n/\delta)}+ n\epsilon_0 \log^2 d\right) \\
        &= \frac{1}{M} \cdot \frac{1+c}{2} M \log M + \cO(1) \\
        &= \frac{1+c}{2} \log M + \cO(1).
    \end{align*}
    So
    \begin{align*}
        \sinh(S) = \Theta(M^{(1+c)/2}).
    \end{align*}

    Next Step: Prove that the test acc is approximately $\Phi(\frac{\sinh(S)}{S\cdot M^{1/2}})$.

\end{proof}

\kaifeng{Trying to extend it to $k$-sparse classification}

Let $\vwref$ be ...

\begin{align*}
    Q_{2/\beta}(\hat{\vw}^\sg) &\ge Q_{2/\beta}(\vwref^\sg) + \inner{\nabla Q_{2/\beta}(\vwref^\sg)}{\hat{\vw}^\sg - \vwref^\sg} \\
    &= Q_{2/\beta}(\vwref^\sg) + \inner{\sum_{i=1}^{n} \lambda_i y_i^* \vx_i^\sg }{\hat{\vw}^\sg - \vwref^\sg}
\end{align*}

\begin{align*}
    \inner{\sum_{i=1}^{n} \lambda_i y_i^* \vx_i}{\hat{\vw} - \vwref} &= 
    \sum_{\substack{i \in [n]: \\ \inne{y_i^* \vx_i}{\vwref} = 1}} \lambda_i\left(\inner{y_i^* \vx_i}{\hat{\vw}} - \inner{y_i^* \vx_i}{\vwref}\right) \\
    &\ge \sum_{\substack{i \in [n]: \\ \inne{y_i^* \vx_i}{\vwref} = 1}} \lambda_i \cdot (1 - 1) = 0.
\end{align*}

\begin{align*}
    Q_{2/\beta}(\hat{\vw}^\ns) &= Q_{2/\beta}(\hat{\vw}) - Q_{2/\beta}(\hat{\vw}^\sg) \\
    &\le Q_{2/\beta}(\vwref) - \left(Q_{2/\beta}(\vwref^\sg) + \inner{\sum_{i=1}^{n} \lambda_i y_i^* \vx_i^\sg }{\hat{\vw}^\sg - \vwref^\sg}\right) \\
    &= -\inner{\sum_{i=1}^{n} \lambda_i y_i^* \vx_i^\sg }{\hat{\vw}^\sg - \vwref^\sg} \\
    &\le \inner{\sum_{i=1}^{n} \lambda_i y_i^* \vx_i^\ns }{\hat{\vw}^\ns}
\end{align*}
