# Supplementary material for: Dichotomy of Early and Late Phase Implicit Biases Can Provably Induce Grokking
Source: arXiv:2311.18817 source file (2024-04-02)
Supplement: Supplementary file 2 [file appendix_prelim.tex]

This section collects some technical results that are used in our analysis.

\begin{lemma}
\label{grad-nuclear}
    ~\cite[Example 2]{watson1992characterization} Let $\bm{A}=\bm{L}\bm{\Sigma}\bm{R}^\top$ be its singular value decomposition, then we have
    \begin{equation}
        \notag
        \partial\|\bm{A}\|_{*} = \left\{ \bm{L}\bm{R}^\top + \bm{E}: \left\|\bm{E}\right\|\leq 1, \bm{L}^\top\bm{E}=0 \text{ and }  \bm{E}\bm{R}=0 \right\}.
    \end{equation}
\end{lemma}
